# Supplementary material for: The Day of the Inductance. Problem of the 7-th Experimental Physics Olympiad, Skopje, 7 December 2019
Source: arXiv:1912.07368 ancillary file (2019-12-28)
Supplement: Supplementary file 1 [file EPO7_ABS-Champion.pdf]

M

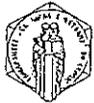

УНИВЕРЗИТЕТ "СВ. КИРИЛ И МЕТОДИЈ"  
ПРИРОДНО МАТЕМАТИЧКИ ФАКУЛТЕТ  
СКОПЈЕ

ИСПИТ ОД ПРЕДМЕТОТ

Кандидат: Димитар Царев

Индекс бр.: \_\_\_\_\_ насока/модул \_\_\_\_\_

Предметот го слушав во: \_\_\_\_\_ семестар 201 \_\_\_\_ год.

Кај наставникот: \_\_\_\_\_

Датум: \_\_\_\_\_

Студентот не смее да ја изнесува  
тетратката од просторијата на испитот.

Не е дозволено истргнување или  
кинење на листови од тетратката.

|    |
|----|
| 1  |
| 2  |
| 3  |
| 4  |
| 5  |
| 6  |
| 7  |
| 8  |
| 9  |
| 10 |

ДЕН 123

спецвалт / Најдобра за теорема

ТМ\*  
РА\*

Шанша

Абсолутна Шанша

5

1.

I 3,53V

II 3,62V

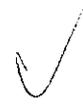

2. 3,0V

3.  $R_{pot} \in (0,00 \text{ k}\Omega, 5,06 \text{ k}\Omega)$   
 $0 \Omega, 5060 \Omega$

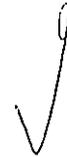

4.

| i | R [ $\Omega$ ] |
|---|----------------|
| 1 | 300            |
| 2 | 380            |
| 3 | 525            |
| 4 | 680            |
| 5 | 820            |
| 6 | 910            |
| 7 | 1001           |

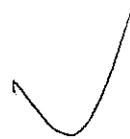

5.

$$\frac{1}{2} V - \frac{1}{3} V = \frac{3-2}{6} V = \frac{1}{6} V = \frac{1}{6} \cdot 1000 \text{ mV} = 166, \overline{6} \text{ mV}$$

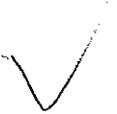

M

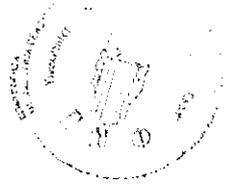

$$(11) \quad z_2 = R_{pot} = 0,22 \text{ k}\Omega = 220 \Omega$$

$$z_2 = 220 \Omega$$

$$(12) \quad z_1 = 300 \Omega$$

$$z_3 = 390 \Omega$$

$$z_4 = 525 \Omega$$

$$\Rightarrow \quad \epsilon = \frac{z_1}{z_2} - \frac{z_4}{z_3} = \frac{300}{220} - \frac{525}{390} = 0,0174$$

$$\boxed{\epsilon = 0,0174} \quad \checkmark$$

Универзитет  
Нови Сад  
Филозофски Факултет

| i  | $z_1 [\Omega]$ | $z_3 [\Omega]$ | $z_4 [\Omega]$ | $R_{pot} [\Omega]$ | $\epsilon [1]$ |
|----|----------------|----------------|----------------|--------------------|----------------|
| 1. | 300            | 390            | 525            | 220                | 0,0174         |
| 2. | 390            | 300            | 680            | 170                | 0,0275         |
| 3. | 300            | 525            | 680            | 230                | 0,0081         |
| 4. | 525            | 390            | 390            | 490                | 0,0125         |
| 5. | 680            | 525            | 320            | 450                | -0,0508        |

✓

$$\epsilon_{\text{cp}} = \frac{\epsilon_1 + \epsilon_2 + \epsilon_3 + \epsilon_4 + \epsilon_5}{5} = 0,0314 \approx 3\%$$

K+K

22.  $R_{pot} = 16,1 \Omega$

$R_L = R_{pot} = 1040 \Omega$

$R_c = 10001 \Omega$

$C = 9,48 \mu F = 9,48 \cdot 10^{-6} F$

$L = C R_L R_c = 9,48 \cdot 10^{-6} \cdot 1040 \cdot 10001 = 9,87 H$

$L = 9,87 H$

| i  | $R_c [\Omega]$ | $R_{pot} [\Omega]$ | $L [H]$ |
|----|----------------|--------------------|---------|
| 1. | 1001           | 1040               | 9,87    |
| 2. | 910            | 1050               | 9,06    |
| 3. | 880            | 1550               | 10,00   |
| 4. | 820            | 1280               | 10,03   |
| 5. | 525            | 1950               | 9,74    |
| 6. | 390            | 2680               | 9,83    |
| 7. | 300            | 3470               | 9,87    |

$L = C R_L R_c$

$R_L = R_{pot}$

$C = 9,48 \cdot 10^{-6} F$

$L_{op} = L_1 + L_2 + L_3 + L_4 + L_5 + L_6 + L_7 = 9,77 H$

$L_{op} = 9,77 H$

Калгугар эд номнаст

L-impedance

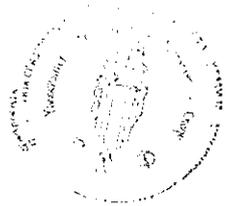

(25)  $U_{AB} = 0$        $\frac{z_1}{z_2} = \frac{z_4}{z_3}$       (condition)

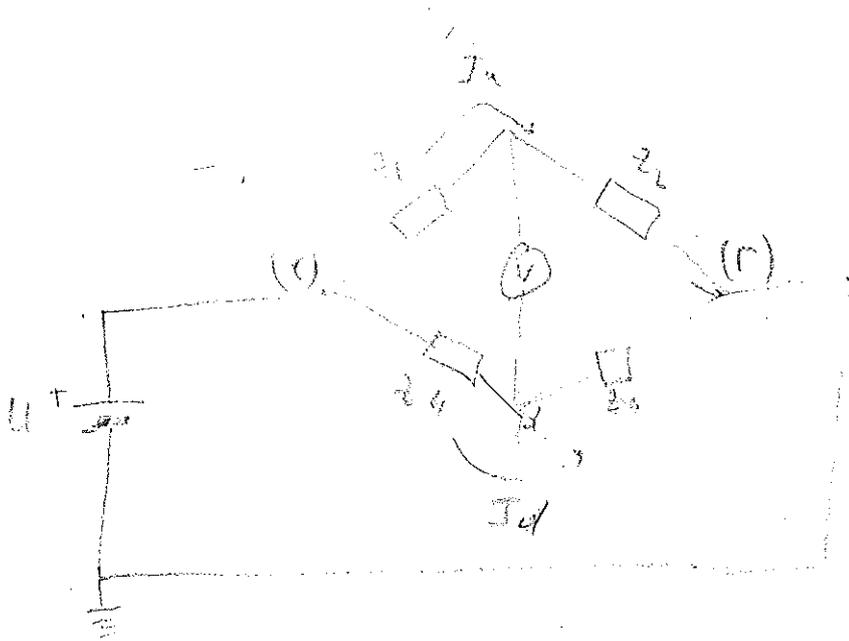

$U_{AB} = 0$

$\Rightarrow$

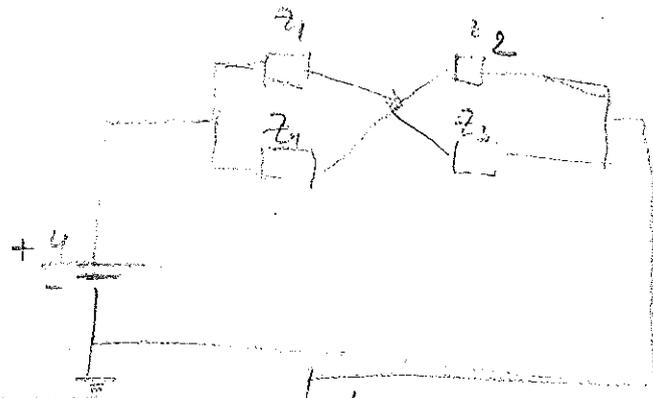

$I_{z_1} = I_{z_2}$

$U_{z_1} = U_{z_4}$

$I_{z_3} = I_{z_4}$

$U_{z_2} = U_{z_3}$

$\left( \begin{array}{l} z_1 \parallel z_4, \quad z_1 \text{ cap. } z_4 \\ z_2 \parallel z_3, \quad z_2 \text{ cap. } z_3 \end{array} \right)$

or  $\Rightarrow \frac{z_1}{z_2} = \frac{\frac{U_{z_1}}{I_{z_1}}}{\frac{U_{z_2}}{I_{z_2}}} = \frac{U_{z_1}}{U_{z_2}} = \frac{U_{z_4}}{U_{z_3}} = \frac{\frac{U_{z_1}}{I_{z_1}}}{\frac{U_{z_3}}{I_{z_3}}} =$

$= \frac{U_{z_4}}{I_{z_4}} = \frac{z_4}{z_3}$

$\Rightarrow \frac{z_1}{z_2} = \frac{z_4}{z_3}$

(24)  $U(t) = U_0 \sin(\omega t)$

$i = i_0 \cos(\omega t)$

$Z_L = R_L = R_{pot} \quad Z_C = R_C$

$Z_1 = Z_L = j\omega L \quad Z_3 = Z_C = \frac{1}{j\omega C}$

$L = C R_C R_L$  Location!

$\frac{Z_1}{Z_2} = \frac{Z_3}{Z_4}$  of (24)

$L = \frac{Z_1}{j\omega} = \frac{Z_2 Z_3}{Z_4 j\omega} = \frac{C \cdot Z_2 Z_3}{Z_4 j\omega C}$   
 $= \frac{C \cdot Z_2 Z_3}{Z_4} \cdot \frac{1}{j\omega} = C Z_2 Z_3 = C R_L R_C$

$\Rightarrow L = C R_L R_C$

(25)

$Z = \frac{U}{I} = \frac{Z_1 Z_3 Z_5}{Z_2 Z_4}$

Location!

$I_3 = I_4 \quad U_0 = 0$

$U_2 = U_5 \quad U_5 = U$

$I_1 = I_2$

By Kirchhoff's current law

$I_3 + I_{Z_1} = I_4$

$I_3 + I_{Z_2} = I_2$

$$I_5 + I_2 = I_4 = I_3 = I_2 = I_1$$

$$I_2 = I_1 + I_4 + I_5$$

$$I = I_2 - I_1 - I_4 = I_5$$

$$\Rightarrow Z = \frac{U}{I} = \frac{U_5}{I_5} = Z_5 = \frac{Z_5 Z_1 Z_2 Z_3 Z_4}{Z_1 Z_2 Z_3 Z_4}$$

$$= \frac{Z_1 \cdot Z_2}{Z_2} \cdot \frac{Z_3 \cdot Z_4}{Z_4} \cdot Z_5 = \boxed{\frac{Z_1 Z_3 Z_5}{Z_2 Z_4}}$$

$$\Rightarrow \boxed{Z = \frac{Z_1 Z_3 Z_5}{Z_2 Z_4}} \quad \checkmark$$

OK

topako

ABS

~~AP Corporates~~
